# Supplementary material for: Symbol-Error Probability Constrained Power Minimization for Reconfigurable Intelligent Surfaces-based Passive Transmitter
Source: arXiv:2311.06900 source file (2023-11-12)
Supplement: Supplementary file 1 [file appendix.tex]

The union-bound SEP constraint functions are in the form of \looseness-1
\begin{align}
    h_k(\boldsymbol{\Theta})=\displaystyle \sum_{\nu=1}^2 \frac{1}{2}\text{erfc}\pc{ {\sqrt{\frac{P}{\sigma_w^2}}}\ \text{tr}\pc{\boldsymbol{\Theta}  \boldsymbol{U}_{\nu,k} } } - p_k.
\end{align}
Considering $P$ as fixed, a sufficient condition to establish convexity is $\nabla^2 h_k(\boldsymbol{\Theta})\succeq \boldsymbol{0}$, \cite[Section 3.1.4]{Boyd_2004}. Taking the derivative of $h_k(\boldsymbol{\Theta})$ with respect to $\boldsymbol{\Theta}$ yields
\begin{align}
\label{eq:grad}
    \frac{\partial h_k(\boldsymbol{\Theta})}{\partial\boldsymbol{\Theta}}=- \sqrt{\frac{P}{\pi\sigma_w^2}}&\sum_{\nu=1}^2 e^{- {\frac{P\cdot \text{tr}\pc{\boldsymbol{\Theta}  \boldsymbol{U}_{\nu,k} }^2}{\sigma_w^2}} } \boldsymbol{U}_{\nu,k}^T .
\end{align}
The Hessian is then computed by taking the derivative with respect to $\boldsymbol{\Theta}^T$ which yields 
\begin{align}
       &\nabla^2{h_k(\boldsymbol{\Theta})}=\frac{2P^{\frac{3}{2}}}{\sqrt{\pi}\sigma_w^3}\sum_{\nu=1}^2 e^{- {\frac{P \cdot \text{tr}\pc{\boldsymbol{\Theta}  \boldsymbol{U}_{\nu,k} }^2}{\sigma_w^2}} } \boldsymbol{U}_{\nu,k}^T\text{tr}\pc{\boldsymbol{\Theta}  \boldsymbol{U}_{\nu,k} } \boldsymbol{U}_{\nu,k}. \notag
\end{align}
With this, one concludes that $h_k(\boldsymbol{\Theta})$ is not convex for all $\boldsymbol{\Theta}\in \mathbb{R}^{2\times N}$. Yet, a sufficient condition for convexity of $h_k(\boldsymbol{\Theta})$ is $\text{tr}\pc{\boldsymbol{\Theta}\boldsymbol{U}_{\nu,k}}\geq0$ for $\nu \in\{1,2\}$.
